# Supplementary material for: VideoStory Embeddings Recognize Events when Examples are Scarce
Source: arXiv:1511.02492 source file (2015-11-08)
Supplement: Supplementary file 1 [file supplementary.pdf]

# Supplementary Materials of VideoStory Embeddings Recognize Events when Examples are Scarce

Amirhossein Habibian, Thomas Mensink, Cees G. M. Snoek

## 1 Introduction

We detail the procedure, which we follow for creating the VideoStory46K dataset [7] by harvesting the Web. This procedure is applicable for collecting the train data needed for learning VideoStory representation, as detailed in the submission. Afterwards, in Section 3, we assess the impact of the quality and quantity of the harvested videos and descriptions on the learned VideoStory representation.

## 2 Harvesting Videos and their Descriptions from the Web

Rather than describing the video content manually, we opt to harvest both the videos and the description from the web. Video sharing web sites, such as YouTube and Vimeo, provide a rich and varied source of videos and user provided descriptions, such as their title captions and comments. Although video title captions do not necessarily correspond to the visual content of the videos, we will show that by harvesting a large number of these captioned videos and applying a set of quality filters we obtain reliable video descriptions.

We start from an initial pool of descriptions, as the collection seeds, and iteratively collect videos and their title captions from YouTube. For the collection seeds, we rely on 3,000 sentence descriptions from the training partition of the NIST TRECVID HAVIC corpus [12]. Then each description within the pool is queried to YouTube and the 25 most relevant videos are retrieved, based on YouTube's textual similarity search. Every retrieved video is passed through a set of quality filters. The videos which pass all the filters are added to the collection and their title captions are added to the description pool. We iteratively repeat this procedure until enough videos are collected. We will first detail our quality filters before providing the statistics of our harvested video and description dataset.

### 2.1 Quality Filters

**Event Filter** Events are generally described by their actors, actions, and possible involved objects [6]. Hence we assume that a description of an event video should contain actors, actions and objects. For this purpose, we parse the grammatical structure of title captions using a probabilistic context free grammar parser [10]. Then we accept a video only if its caption includes verbs, subjects, and objects.

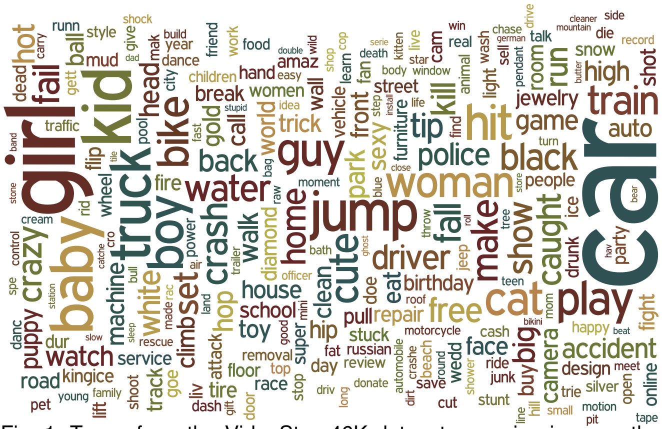


Fig. 1. Terms from the VideoStory46K dataset occurring in more than 500 title captions of the harvested YouTube videos.

**Visualness Filter** There are many terms in title captions which do not refer to visually depictable attributes, such as `buy`, `God`, and `genius`. These attributes are not recognizable by present-day visual classifiers, so should not be included in the collection. For this filter we evaluate the visualness of caption terms. Rather than relying on visual features [3], [5], [11], which are expensive to extract and limit the scalability, we evaluate the visualness of each term in the title caption by measuring its similarities to the ImageNet synsets [4] in the WordNet hierarchy. We measure the similarity of each synset pair by following [2], which finds overlaps between the glosses of two synsets as well as their directly linked synsets. Finally, we define the visualness of a title caption by averaging the visualness of all its terms. The captions whose visualness exceeds a threshold of 0.5 are accepted by our harvesting procedure.

**Reality Filter** A considerable amount of YouTube videos are related to celebrities, TV series, and movie trailers. We observe these professional videos are typically semantically dissimilar to the event videos which we are interested in. Moreover, they often infringe intellectual property rights. Therefore, we prefer to filter out the corresponding videos and title captions. Our reality filter relies on a list of keywords from Wikipedia, which provides an extensive index

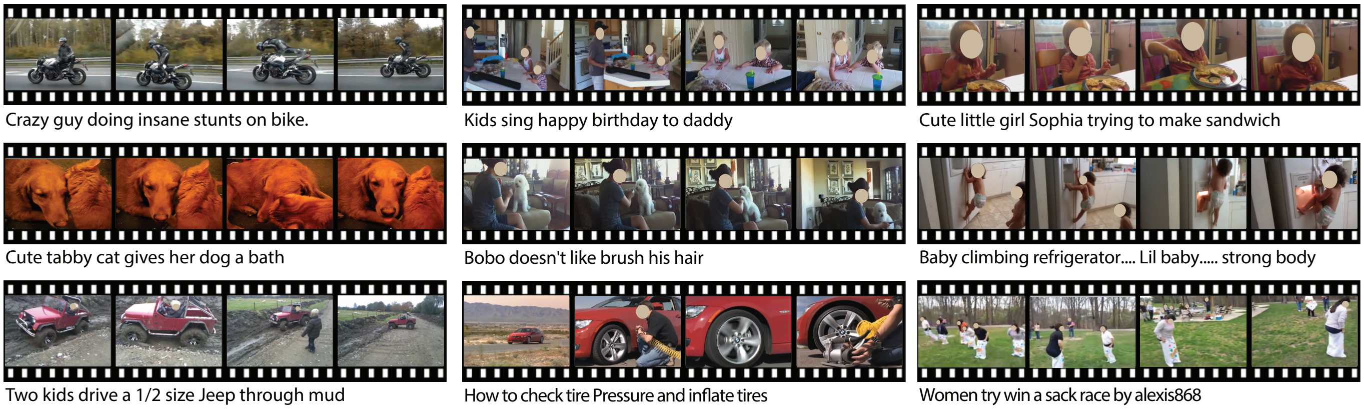


Fig. 2. Example videos and title captions from our introduced VideoStory46K dataset.

of celebrity, TV series and movie names[1]. We exclude the videos whose description matches any of the keywords from the list.

**Temporal Filter** Our last filter rests on the assumption that short videos better match their title captions, compared to long videos. It is because long videos usually contain a broad set of attributes that are typically not specified completely by their captions. Hence, we only retrieve the YouTube videos which are shorter than 120 seconds.

### 2.2 VideoStory46K Dataset

Following the proposed procedure, including all quality filters, we harvest 45,826 videos from YouTube. The videos have an average length of 58.4 seconds and the whole collection contains 743 hours of videos. Every video comes with a short title caption provided by the user who has uploaded the video. Every caption is made of 7.7 individual terms on average, with a standard deviation of 1.8 terms. There are 19,159 unique terms in the captions, most of them occurring infrequently in the collection, *i.e.*, 50% of the terms occur only once in the collection, and only 0.4% of the terms occur more than 500 times (see Figure 3.). Some examples of these frequent terms are shown as a tag cloud in Figure 1. Our dataset of videos and their descriptions, which we call VideoStory46K, is available for download at http://www.mediamill.nl. Illustrative examples from the dataset are shown in Figure 2.

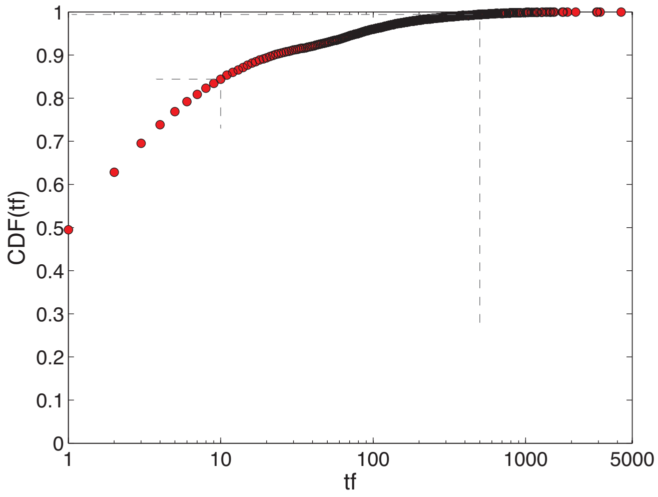


Fig. 3. Cumulative distribution function (CDF) for term frequencies in the title captions of the VideoStory46K dataset. The y-axis shows the cumulative probability that a term occurs in the caption, the x-axis denotes the term frequency $tf$ in logarithmic scale. It shows that most of the terms rarely occur in captions *e.g.*, 50% (resp. 84%) of the terms only occur in 1 (resp. 10) captions.

## 3 Experiment on Description Quality and Quantity

We assess the influence of the quality and quantity of the videos and descriptions that we use as input to learn our VideoStory. We compare the VideoStory learned from the VideoStory46K dataset with two baselines.

1. ***ExpertSentences10K***, includes 10K videos from the Research partition of the NIST TRECVID HAVIC corpus [8], [12]. Each video in this collection comes with an expert written description per video. The descriptions are made of a few sentences written by a team of 60 expert annotators with the purpose of summarizing the visual content of the videos. Consequently, there is always a strong correspondence between a description and its video in this collection.

2. ***VideoStory10K***, includes 10K random videos and descriptions from the VideoStory46K dataset, which we collected as discussed in Section 2. This collection includes the same number of videos and captions as the ExpertSentences10K dataset, but the captions are generally of lower quality for event recognition because of the non-expert descriptions and the fact that video captions on YouTube do not necessarily correspond to the visual content.

**Experimental Setup.** The experiments are performed on three test sets: MED and Kindred from the TRECVID Multimedia Event Detection [1], [12] and the Columbia Consumer Video (CCV) [9], by following the standard data partitioning [7]. We rely on the MBH descriptors along the motion trajectories [13] to extract the low-level video representation as detailed in Section 4.2 in the submission. We use a varying dimensionality of the representation, starting from 32 up to 2,048, and we compare their effectiveness for recognizing

1. wikipedia.org/wiki/List_of_American_television_series

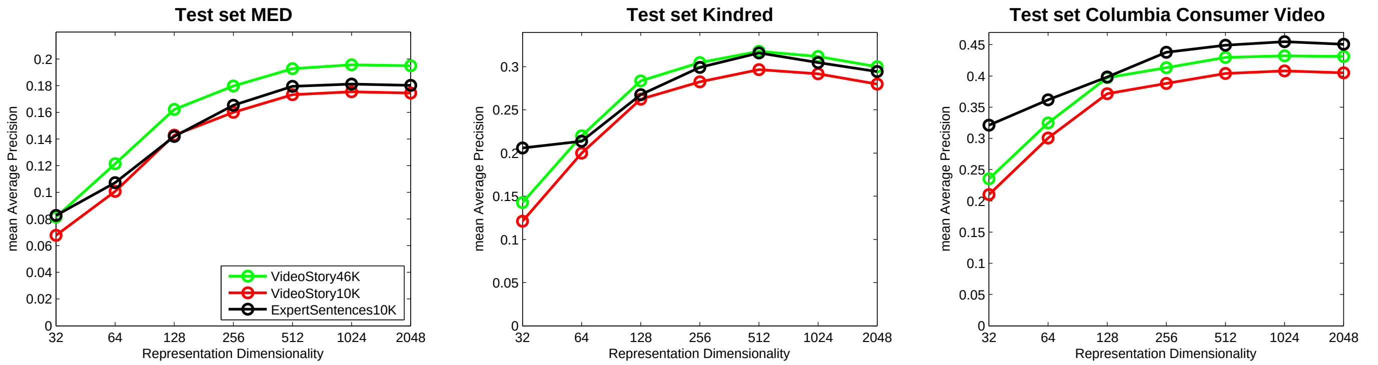


Fig. 4. Description quality and quantity. As expected, the more reliable the correspondence between description and video content, the better the result. The event recognition accuracy obtained by ExpertSentences10K can be approached, and even improved, by simply harvesting more descriptions from the web.

events from few examples.

**Results.** The results are presented in Figure 4. As expected, the more reliable the correspondence between the description and the video content it describes, the better the result. A VideoStory learned from ExpertSentences10K always performs better than an embedding learned from the same amount of descriptions from VideoStory10K. Yet it should be noted that the expert descriptions are generally unavailable or hard to obtain. Interestingly, the event recognition accuracy obtained by expert descriptions can be approached, and even improved (for both the test set MED and test set Kindred) by simply harvesting more descriptions from the web. When considering all results, the complete VideoStory46K dataset is the best choice overall. The embedding reduces the influence of noisy video descriptions, especially when the number of input videos and descriptions are large. It demonstrates the value of user generated videos and descriptions as an unlimited, free, yet precious resource for constructing an effective VideoStory.

## References


[1] M. Akbacak, R. Bolles, J. Burns, M. Eliot, A. Heller, J. Herson, G. Myers, R. Nallapati, S. Pancoast, J. van Hout, et al. The 2012 sesame multimedia event detection (med) system. In *TRECVID*, 2012. 3

[2] S. Banerjee and T. Pedersen. Extended gloss overlaps as a measure of semantic relatedness. In *IJCAI*, 2003. 2.1

[3] T. L. Berg, A. C. Berg, and J. Shih. Automatic attribute discovery and characterization from noisy web data. In *ECCV*, 2010. 2.1

[4] J. Deng, W. Dong, R. Socher, L.-J. Li, K. Li, and L. Fei-Fei. ImageNet: A large-scale hierarchical image database. In *CVPR*, 2009. 2.1

[5] J. Dodge et al. Detecting visual text. In *NAACL*, 2012. 2.1

[6] S. Guadarrama et al. Youtube2text: Recognizing and describing arbitrary activities using semantic hierarchies and zero-shot recognition. In *ICCV*, 2013. 2.1

[7] A. Habibian, T. Mensink, and C. G. Snoek. Videostory: A new multimedia embedding for few-example recognition and translation of events. In *ACM MM*, 2014. 1, 3

[8] A. Habibian and C. G. Snoek. Video2sentence and vice versa. In *ACM MM*, 2013. 3

[9] Y.-G. Jiang, G. Ye, S.-F. Chang, D. Ellis, and A. Loui. Consumer video understanding: A benchmark database and an evaluation of human and machine performance. In *ICMR*, 2011. 3

[10] D. Klein and C. Manning. Accurate unlexicalized parsing. In *Association for Computational Linguistics*, 2003. 2.1

[11] P. Kuznetsova, V. Ordonez, A. Berg, T. Berg, and Y. Choi. Generalizing image captions for image-text parallel corpus. In *Association for Computational Linguistics*, 2013. 2.1

[12] S. Strassel et al. Creating havic: Heterogeneous audio visual internet collection. In *LREC*, 2012. 2, 3, 3

[13] H. Wang and C. Schmid. Action recognition with improved trajectories. In *ICCV*, 2013. 3
